# Supplementary material for: Measurement of the charm mixing parameter $y_{CP} - y_{CP}^{K\pi}$ using two-body $D^0$ meson decays
Source: arXiv:2202.09106 source file (2022-05-30)
Supplement: Supplementary file 1 [file 10_supplementary.tex]

\clearpage

\section{Supplementary material}
\label{sec:Supplementary-App}

Figures \ref{fig:yCP_kinematics_P} and \ref{fig:yCP_kinematics_eta} present the improvement of the $p(D^0)$ and $\eta(D^0)$ distributions following both kinematic matching and weighting procedures. Figures~\ref{fig:yCP_Full_Run2_supp}~and~\ref{fig:yCP_Full_pGun} show the results of the measurements of the analysis with data and simulation, respectively. Figures~\ref{fig:yCP_kinematics_RapidSim} and \ref{fig:yCP_RapidSim} present the improvement of $p(D^0)$, $\eta(D^0)$ and $R^{KK}(t)$ following the kinematic matching procedure with fast simulation. Figure~\ref{fig:yCP_CC_allYears_Run2} presents the measurement of $\ycp^{CC}$ with the full Run~2 data set. Figure~\ref{fig:yCP_WA_NEW} shows the updated world average value of $\ycp - \ycp^{K\pi}$. Figures~\ref{fig:gammacombo_x_y}, \ref{fig:gammacombo_Delta_Kpi_y}, \ref{fig:gammacombo_y} and \ref{fig:gammacombo_Delta_Kpi} display the improvement of charm mixing parameters with the measurement of this paper.

\begin{figure}[b]
\centering
\begin{minipage}[b]{0.45\textwidth}
\includegraphics[width=1.\textwidth]{figs-supplementary/Fig8a.pdf}
\end{minipage}
\begin{minipage}[b]{0.45\textwidth}
\includegraphics[width=1.\textwidth]{figs-supplementary/Fig8b.pdf}
\end{minipage}
\begin{minipage}[b]{0.45\textwidth}
\includegraphics[width=1.\textwidth]{figs-supplementary/Fig8c.pdf}
\end{minipage}
\begin{minipage}[b]{0.45\textwidth}
\includegraphics[width=1.\textwidth]{figs-supplementary/Fig8d.pdf}
\end{minipage}
\begin{minipage}[b]{0.45\textwidth}
\includegraphics[width=1.\textwidth]{figs-supplementary/Fig8e.pdf}
\end{minipage}
\begin{minipage}[b]{0.45\textwidth}
\includegraphics[width=1.\textwidth]{figs-supplementary/Fig8f.pdf}
\end{minipage}
\caption{(Left) normalised distributions of the $\Dz$ momentum in the raw condition, and (right) following both kinematic matching and weighting procedures. The distributions are shown for the (top) $\ycp^{CC}$, (middle) $\ycp^{\pi\pi} - \ycp^{K\pi}$ and (bottom) $\ycp^{KK} - \ycp^{K\pi}$ measurements. The plots are obtained with the 2017 \textit{MagUp} sample.}
\label{fig:yCP_kinematics_P}
\end{figure}

\begin{figure}[tb]
\centering
\begin{minipage}[b]{0.49\textwidth}
\includegraphics[width=1.\textwidth]{figs-supplementary/Fig9a.pdf}
\end{minipage}
\begin{minipage}[b]{0.49\textwidth}
\includegraphics[width=1.\textwidth]{figs-supplementary/Fig9b.pdf}
\end{minipage}
\begin{minipage}[b]{0.49\textwidth}
\includegraphics[width=1.\textwidth]{figs-supplementary/Fig9c.pdf}
\end{minipage}
\begin{minipage}[b]{0.49\textwidth}
\includegraphics[width=1.\textwidth]{figs-supplementary/Fig9d.pdf}
\end{minipage}
\begin{minipage}[b]{0.49\textwidth}
\includegraphics[width=1.\textwidth]{figs-supplementary/Fig9e.pdf}
\end{minipage}
\begin{minipage}[b]{0.49\textwidth}
\includegraphics[width=1.\textwidth]{figs-supplementary/Fig9f.pdf}
\end{minipage}
\caption{(Left) normalised distributions of the $\Dz$ pseudorapidity in the raw condition, and (right) following both kinematic matching and weighting procedures. The distributions are shown for the (top) $\ycp^{CC}$, (middle) $\ycp^{\pi\pi} - \ycp^{K\pi}$ and (bottom) $\ycp^{KK} - \ycp^{K\pi}$  measurements. The plots are obtained with the 2017 \textit{MagUp} sample.}
\label{fig:yCP_kinematics_eta}
\end{figure}

\begin{figure}
\centering
\begin{minipage}[b]{0.59\textwidth}
\includegraphics[width=1.\textwidth]{figs-supplementary/Fig10a.pdf}
\end{minipage}
\begin{minipage}[b]{0.59\textwidth}
\includegraphics[width=1.\textwidth]{figs-supplementary/Fig10b.pdf}
\end{minipage}
\begin{minipage}[b]{0.59\textwidth}
\includegraphics[width=1.\textwidth]{figs-supplementary/Fig10c.pdf}
\end{minipage}
\caption{Results for (top) $\ycp^{CC}$, (centre) $\ycp^{\pi\pi} - \ycp^{K\pi}$ and (bottom) $\ycp^{KK} - \ycp^{K\pi}$. The measurements employing raw data, and following the kinematic matching and both matching and weighting conditions are shown in green, blue and red, respectively, and are obtained by fitting with an exponential model. The measurements in purple employ the fit model of where the presence of secondary decays is considered.
In the y-axis labels, the data-taking year is abbreviated with the last two digits only and the magnet polarity \MagUp (\MagDown) is abbreviated as ``Up'' (``Dw''). The results for each condition on the right side of each plot are weighted averages, $\chi^2$ and numbers of degrees of freedom ($\mathrm{NDF}$) determined from a constant $\chi^2$ fit to each individual value. The uncertainties are only statistical.}
\label{fig:yCP_Full_Run2_supp}
\end{figure}

\begin{figure}[tb]
\centering
\begin{minipage}[b]{0.59\textwidth}
\includegraphics[width=1.\textwidth]{figs-supplementary/Fig11a.pdf}
\end{minipage}
\begin{minipage}[b]{0.59\textwidth}
\includegraphics[width=1.\textwidth]{figs-supplementary/Fig11b.pdf}
\end{minipage}
\begin{minipage}[b]{0.59\textwidth}
\includegraphics[width=1.\textwidth]{figs-supplementary/Fig11c.pdf}
\end{minipage}
\caption{Results for (top) $\ycp^{CC}$, (centre) $\ycp^{\pi\pi} - \ycp^{K\pi}$ and (bottom) $\ycp^{KK} - \ycp^{K\pi}$, obtained with simulation. The measurements under the raw condition, and following the kinematic matching and both kinematic and reweighting conditions are shown in green, blue and red, respectively, and are obtained by fitting with an exponential model. The uncertainties are only statistical.}
\label{fig:yCP_Full_pGun}
\end{figure}

\begin{figure}[b]
\centering
\begin{minipage}[b]{0.49\textwidth}
\includegraphics[width=1.\textwidth]{figs-supplementary/Fig12a.pdf}
\end{minipage}
\begin{minipage}[b]{0.49\textwidth}
\includegraphics[width=1.\textwidth]{figs-supplementary/Fig12b.pdf}
\end{minipage}
\begin{minipage}[b]{0.49\textwidth}
\includegraphics[width=1.\textwidth]{figs-supplementary/Fig12c.pdf}
\end{minipage}
\begin{minipage}[b]{0.49\textwidth}
\includegraphics[width=1.\textwidth]{figs-supplementary/Fig12d.pdf}
\end{minipage}
\caption{(Left) normalised distributions of the $\Dz$  (top) momentum and (bottom) pseudorapidity in the raw condition, and (right) following the kinematic matching procedure. The plots are obtained with fast simulation.}
\label{fig:yCP_kinematics_RapidSim}
\end{figure}

\begin{figure}[b]
\centering
\begin{minipage}[b]{0.49\textwidth}
\includegraphics[width=1.\textwidth]{figs-supplementary/Fig13a.pdf}
\end{minipage}
\begin{minipage}[b]{0.49\textwidth}
\includegraphics[width=1.\textwidth]{figs-supplementary/Fig13b.pdf}
\end{minipage}
\caption{Decay-time ratios $R^{KK}(t)$ (left) in the raw condition and (right) following the kinematic matching procedure. The solid lines correspond to fits performed to determine $\ycp^{KK} - \ycp^{K\pi}$. The plots are obtained with fast simulation.}
\label{fig:yCP_RapidSim}
\end{figure}

\begin{figure}[tb]
\centering
\includegraphics[width=0.6\textwidth]{figs-supplementary/Fig14.pdf}
\caption{Distribution of $R^{CC}(t)$ using the full \lhcb Run~2 data set, with the result of $\ycp^{CC}$ overlaid in blue.}
\label{fig:yCP_CC_allYears_Run2}
\end{figure}

\begin{figure}
    \centering
    \includegraphics[width=\textwidth]{figs-supplementary/Fig15.pdf}
    \caption{Updated world average value of $\ycp - \ycp^{K\pi}$\cite{Aitala:1999dt,Link:2000cu,Csorna:2001ww,Zupanc:2009sy,LHCb-PAPER-2011-032,Lees:2012qh,Ablikim:2015hih,Staric:2015sta,LHCb-PAPER-2018-038,Nayak:2019byo}. The first uncertainties are statistical and the second systematic. The measurement of this paper is denoted as \textit{\lhcb 2021}. The inset plot shows the measurements in a reduced horizontal range and with a compressed vertical scale.
The $\chi^2/\mathrm{NDF}$ value of the world average fit is measured as $10.9/10$, corresponding to a probability of $36.3\%$.}
    \label{fig:yCP_WA_NEW}
\end{figure}

\begin{figure}
    \centering
    \includegraphics[width=0.75\textwidth]{figs-supplementary/Fig16.pdf}
    \caption{Profile likelihood contours of $y$ versus $x\equiv (m_1-m_2)/\Gamma$ of the (light blue) \lhcb Charm Only and (dark blue) \lhcb Beauty and Charm  combinations~\cite{LHCb-PAPER-2021-033}, and of (red) the measurement of this paper. In the latter, $x_D$ is fixed to the global best fit, where one can see that the improvements on $y$ from this measurement and the Beauty and Charm combinations are compatible and similar in size.  
    The contours indicate the $68\%$ and $95\%$ confidence region.}
    \label{fig:gammacombo_x_y}
\end{figure}

\begin{figure}
    \centering
    \includegraphics[width=0.75\textwidth]{figs-supplementary/Fig17.pdf}
    \caption{Profile likelihood contours of $y$ versus $\delta_{K\pi}$. The combination of (red) \lhcb Charm Only results with the measurement of this paper is compared to (dark blue) the \lhcb Beauty and Charm combination~\cite{LHCb-PAPER-2021-033}, indicating similar improvements with respect to (light blue) the \lhcb Charm Only combination. The orange band is produced fixing $x_D$ and $R_D$ to the global best fit.}
    \label{fig:gammacombo_Delta_Kpi_y}
\end{figure}

\begin{figure}
    \centering
    \includegraphics[width=0.75\textwidth]{figs-supplementary/Fig18.pdf}
    \caption{One dimensional $\mathrm{1-CL}$ profiles of $y$ as for the (light blue) \lhcb Charm Only  and  (dark blue) \lhcb Beauty and Charm combinations~\cite{LHCb-PAPER-2021-033}, and for (red)  the Charm Only combination including the measurement of this paper.}
    \label{fig:gammacombo_y}
\end{figure}

\begin{figure}
    \centering
    \includegraphics[width=0.75\textwidth]{figs-supplementary/Fig19.pdf}
    \caption{One dimensional $\mathrm{1-CL}$ profiles of $\delta_{K\pi}$ as for the (light blue) \lhcb Charm Only  and (dark blue) \lhcb Beauty and Charm combinations~\cite{LHCb-PAPER-2021-033}, and for  (red)  the Charm Only combination including the measurement of this paper.}
    \label{fig:gammacombo_Delta_Kpi}
\end{figure}

\clearpage
